# Supplementary material for: Infinite-Fidelity Coregionalization for Physical Simulation
Source: arXiv:2207.00678 source file (2022-10-23)
Supplement: Supplementary file 1 [file suppl.tex]

\section*{Data Generation Details}

\noindent \textbf{Burgers' equation} is a canonical nonlinear hyperbolic PDE, widely used to model various physical phenomena, such as nonlinear acoustics~\citep{sugimoto1991burgers},  fluid dynamics~\citep{chung2010computational},  and traffic flows~\citep{nagel1996particle}. Due to its capability of developing discontinuities  (\ie shock waves), Burger's equation is used as a benchmark test example for many numerical solvers and surrogate models~\citep{kutluay1999numerical,shah2017reduced,raissi2017physics}.The viscous version of Burger's equation is given by 
\[
\frac{\partial u}{\partial t} + u \frac{\partial u}{\partial x} = v \frac{\partial^2 u}{\partial x^2},
\]
where $u$ is the volume, $x$ is a spatial location, $t$ is the time, and $v$ is the viscosity. We set $x\in[0,1]$, $t \in [0,3]$, and $u(x,0)=\sin(x\pi/2)$ with a homogeneous Dirichlet boundary condition.  The input parameter is the viscosity $v \in [0.001, 0.1]$. Given the input, we aim to predict the solution field (\ie the values of $u$) in the spatial-temporal domain $[0, 1] \times [0, 3]$. To obtain the training and test datasets, we solve the equation using the finite element~\citep{zienkiewicz1977finite} with hat functions in space and backward Euler in time domains on a regular mesh. 

\noindent \textbf{Poisson's equation} is an elliptic PDE and commonly used to model potential fields, \eg  electrostatic and gravitational fields, in physics and mechanical engineering~\citep{chapra2010numerical}. The equation used in our experiment is given by
\[
\Delta u = \beta \delta(\x - \c),
\]
where $\Delta $ is the Laplace operator~\citep{persides1973laplace}, $\u$ is the volume, $\delta(\cdot)$ is the Dirac-delta function, and $\c$ is the center of the domain. We  used a 2D spatial domain, $\x \in [0, 1] \times [0, 1$], and Dirichlet boundary conditions. We used  the constant values of the four boundaries and $\beta$ as the input parameters, each of which ranges from $0.1$ to $0.9$. We solved the equation using the finite difference method with the first order center differencing scheme and regular rectangle meshes.

\noindent \textbf{Heat equation} is a fundamental PDE that models heat conduction over time. It is also widely used in many other areas, such as probability theory~\citep{spitzer1964electrostatic,burdzy2004heat} and financial mathematics~\citep{black1973pricing}. 
%Hence, it is also widely used as a surrogate model  ~\citep{efe2003proper,raissi2017machine}.
The equation is defined as
\[
\frac{\partial u}{\partial t} + \alpha \Delta u =0,
\]  
where $u$ is the heat, $\alpha$ the thermal conductivity, and $\Delta$ the Laplace operator. In our experiment, we used  a 2D spatial-temporal domain $x\in[0,1]$, $t \in [0,5]$ with the Neumann boundary condition at $x=0$ and $x=1$, and $u(x,0)=H(x-0.25)-H(x-0.75)$, where $H(\cdot)$ is the Heaviside step function. We considered three input parameters ---  the flux rate $\in [0, 1]$ of the left boundary at $x=0$, the flux rate $\in [-1, 0]$ of the right boundary at $x=1$, and $\alpha \in [0,01, 0.1]$.% (ranging from 0.01 to 0.1).
To generate the training and test examples, we solve the equation with the finite difference in the space domain and backward Euler in the time domain.

\subsection{Predicting Fluid Dynamics}\label{sect:appendix:fluid}
We also examined \ours in predicting the velocity field of a flow within a rectangular domain with a prescribed velocity along the boundaries~\citep{bozeman1973numerical}. This is a classical computational fluid dynamics (CFD) problem. The simulation of the flow involves solving the incompressible Navier-Stokes (NS) equation~\citep{chorin1968numerical}, 
\[
\rho (\textbf{u} \cdot \nabla) \textbf{u} = -\nabla p + \mu \nabla^2 \textbf{u},
\]
where $\rho$ is the density, $p$ is the pressure, $\textbf{u}$ is the velocity, and $\mu$ is the dynamic viscosity. The equation is well known to be challenging to solve due to their complicated behaviours under large Reynolds numbers.% (defined by $\rho$, $\u$, $\mu$, \etc).
We set the rectangular domain to $[0, 1] \times [0, 1]$, and time $t \in [0, 10]$. 
The input includes the tangential velocities of the four boundaries and the Reynold number $\in [100, 5000]$. The output are the first component of the velocity field at $20$ equally spaced time steps in $[0, 10]$ (see Fig. \ref{fig:cfd-example}). To generate the training and test examples, we used the SIMPLE algorithm~\citep{caretto1973two} with a stagger grid~\citep{versteeg2007introduction}, the up-wind scheme~\citep{versteeg2007introduction} for the spatial difference, and the implicit time scheme with fixed time steps to solve the NS equation.
